# Supplementary material for: The inner solar system cratering record and the evolution of impactor populations
Source: arXiv:1407.4521 source file (2014-07-16)
Supplement: Supplementary file 1 [file Appendix-TableA1.pdf]

# Appendix

## Table A-1: References and Notes for Crater Data

| Craters Description | Reference(s) | Figures(s) | Notes |
|---|---|---|---|
| Lunar Highlands craters | Arthur et al., 1963 | 1,3,4,5,7,9,10,12, 13,15,16 | Lunar front-side highlands |
| Lunar Class 1 craters | Strom, 1977; Arthur et al., 1963 | 4,6 | These are both highland and Mare craters. |
| Lunar Copernican and Eratosthenian | Wilhelms et al., 1978. | 4,12,16 | These are post-mare craters identified both morphologically and stratigraphically |
| Lunar Post-Mare | Strom, 1977; Arthur et al., 1963 | 4,16 | Lunar Front-side Maria |
| Lunar Post-Orientale | This work | 16 | Counts on Lunar Reconnaissance Orbiter Camera WAC images |
| Lunar Bruno | Xiao & Strom, 2012 | 11 | |
| Mercury Heavily Cratered | Strom et al., 2008; Strom, 1977 | 1 | These counts are from the heavily crater terrain from Mariner 10 incoming, outgoing and south polar areas. |
| Mercury Heavily Cratered High Density | Strom et al., 2011 | 7 | This area is a region from area with one of the highest crater densities on Mercury |
| Mercury Northern Plains | Ostrach, et al., 2011 | 6 | These counts are the entire Northern Plains from MESSENGER images |
| Mercury Caloris Exterior Plains | Strom et al., 2008, 2011 | 6,10 | These counts are from MESSENGER's first flyby and Mariner 10's second encounter. |
| Mercury Class 1 | This work | 6,12 | Same morphological Class as lunar Class 1 craters |

# Appendix
## Table A-1: References and Notes for Crater Data

| | | | |
|---|---|---|---|
| Venus Production | Strom et al, 1994 | 8,12 | These data come from the catalog of Venus craters by Schaber and Strom |
| Venus Screened | Strom et al, 1994 | 8 | As above |
| Venus Multi-Screened | Strom et al, 1994 | 8 | As above |
| Mars Highlands | Strom et al., 1992 | 9,15 | These counts are from the most heavily craters regions on Mars as compiled by Barlow |
| Mars Old Cratered Plains | Strom et al., 1992 | 9,12 | Moderately cratered plains east of Tharsis partly including the geologic unit "Old Volcanic Material" |
| Mars Northern Plains | Strom et al., 1992 | 9 | This area is largely Vastitas Borealis including the geologic unit "Mottled Plains Unit" |
| Mars Hellas Plains | Strom et al., 1992 | 9 | Plains within the Hellas Basin |
| Mars Tharsis Plains | Strom et al., 1992 | 9 | Plains surrounding the Tharis volcanic constructs |
| Mars Young Plains | Strom et al., 2005 | 10,11,12 | Plains associated with Tharsis |
| Mars small rayed craters | This work | 11 | Rayed craters from Viking orbital images |
| Callisto and Ganymede | Strom et al. 1981 | 13 | |
| Rhea and Tethys | This work | 13 | Previously Unpublished |
| Ariel, Miranda and Titania | Greenberg et al, 1991 | 13 | |
| Triton | Strom et al., 1990 | 13 | |
